# Supplementary material for: Interacting Hopf Algebras: the theory of linear systems
Source: arXiv:1805.03032 source file (2018-05-04)
Supplement: Supplementary file 1 [file appendixSpanF.tex]

\begin{lemma}\label{lemma:mirrorcube} Let the following be a commutative cube where $\pi_n, \pi_m,\pi_r,\pi_z$ are permutations.
\begin{eqnarray*}
\xymatrix@=15pt{
& n_1 \ar[rr]^{q_1} \ar[dd]_<<<<<<<<<<<{\pi_n} & & z_1 \ar[dd]^{\pi_z} \\
r_1 \ar[ur]^{g_1} \ar[rr]^<<<<<<<<<<<<<{f_1} \ar[dd]_{\pi_r} & & m_1 \ar[ur]^>>>>>>>{p_1} \ar[dd]_<<<<<<<<<<<{\pi_m}& \\
& n_2 \ar[rr]^<<<<<<<<<<<<<{q_2} & & z_2 \\
r_2 \ar[ur]^{g_2} \ar[rr]^{f_2} & & m_2 \ar[ur]_{p_2} & \\
}
\end{eqnarray*}
Then the equation associated with the top face and the one associated with the bottom face are equivalent in $\F + \Fop$, that is:
\begin{eqnarray*}
\lower10pt\hbox{\includegraphics[width=3cm]{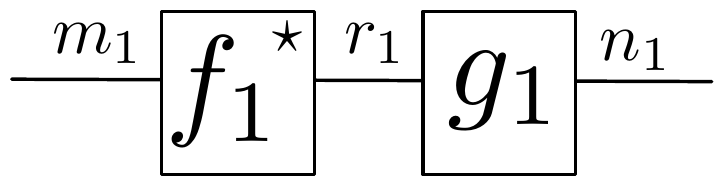}} =
\lower10pt\hbox{\includegraphics[width=3cm]{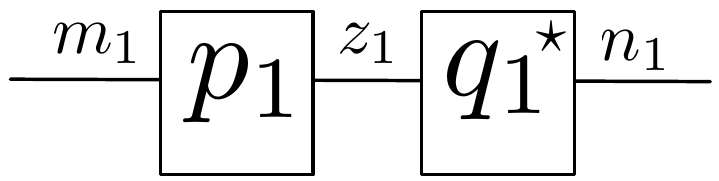}} & \qquad \text{iff} \qquad &
\lower10pt\hbox{\includegraphics[width=3cm]{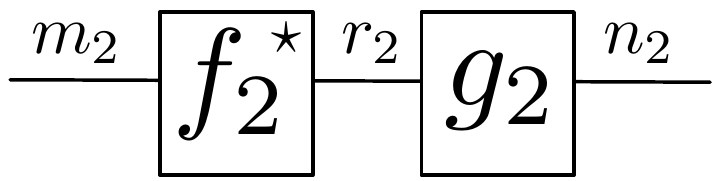}} =
\lower10pt\hbox{\includegraphics[width=3cm]{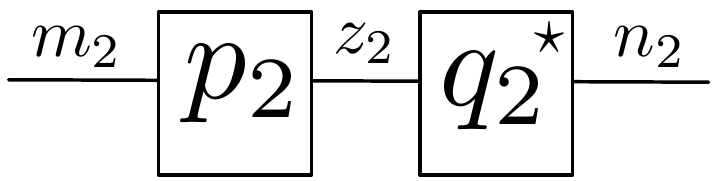}}
\end{eqnarray*}
\end{lemma}
\begin{proof} See derivation on scanned notes. \end{proof}

Lemma \ref{lemma:mirrorcube} is crucial for all the next proofs as it tells us that the equational theory of $\F + \Fop$ does not distinguish between different ways of constructing diagrams of $\F$ which are unique only up-to isomorphisms (= up-to permutations). In particular, it will allow us to always assume that pullbacks are of a suitable shape.

\begin{lemma} \label{lemma:pbcoproductprovable} Let the following be a commutative diagram, where each horizontal face is a pullback and the columns are all coproduct injections.
\begin{eqnarray*}
\xymatrix@=15pt{
& n_1 \ar[rr]^{q_1} \ar[dd] & & z_1 \ar[dd] \\
r_1 \ar[ur]^{g_1} \ar[rr]^<<<<<<<<<<<<<{f_1} \ar[dd] & & m_1 \ar[ur]^>>>>>>>{p_1} \ar[dd] & \\
& n_3 \ar[rr]^<<<<<<<<<<<<<{q_3} & & z_3 \\
r_3 \ar[ur]^{g_3} \ar[rr]^<<<<<<<<<<<<<{f_3} & & m_3 \ar[ur]_{p_3} & \\
& n_2 \ar[uu] \ar[rr]^<<<<<<<<<<<<<{q_2} & & z_2 \ar[uu] \\
r_2 \ar[ur]^{g_2} \ar[rr]^{f_2} \ar[uu] & & m_2 \ar[ur]_{p_2} \ar[uu] & \\
}
\end{eqnarray*}
If both the equation associated with the topmost and with the bottommost pullback are provable, then also the one associated with the middle pullback is also provable. That is, if
\begin{eqnarray*}
\lower10pt\hbox{\includegraphics[width=3cm]{graffles/f1g1.pdf}} =
\lower10pt\hbox{\includegraphics[width=3cm]{graffles/p1q1.pdf}} & \qquad \text{and} \qquad &
\lower10pt\hbox{\includegraphics[width=3cm]{graffles/f2g2.pdf}} =
\lower10pt\hbox{\includegraphics[width=3cm]{graffles/p2q2.pdf}}
\end{eqnarray*}
then
\begin{eqnarray*}
\lower10pt\hbox{\includegraphics[width=3cm]{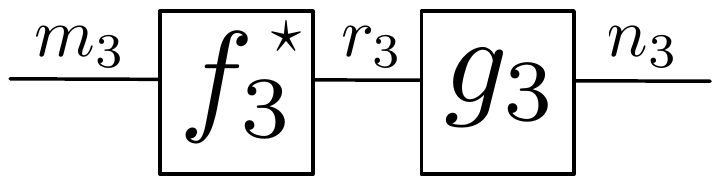}} =
\lower10pt\hbox{\includegraphics[width=3cm]{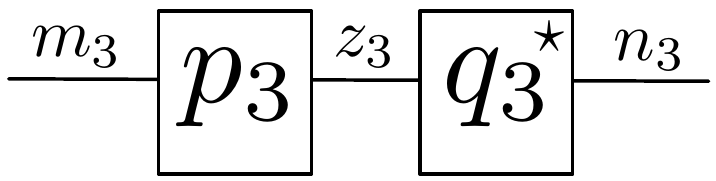}}
\end{eqnarray*}
\end{lemma}
\begin{proof} Let $i_1 \: m_1 \to m_3$ and $i_2 \: m_2 \to m_3$ denote the coproduct injections into $m_3 = m_1 + m_2$. By definition $f_1 \tns f_2 = [f_1 \poi i_1 , f_2 \poi i_2] \: r_3 \to m_3$ is given by the universal property of $r_3 = r_1 + r_2$ and thus by uniqueness $f_1 \tns f_2 = f_3$. In a similar way, we have $g_3 = g_1 \tns g_2$, $q_3 = q_1 \tns q_2$ and $p_3 = p_1 \tns p_2$. This means that the middle pullback is equal to the following diagram
\begin{eqnarray}\label{eq:tensoredpb}
\xymatrix@=15pt{
& n_1 + n_2 \ar[rr]^<<<<<<<<<<<<<{q_1 \tns q_2} & & z_1 + z_2 \\
r_1 + r_2 \ar[ur]^{g_1 \tns g_2} \ar[rr]^{f_1 \tns f_2} & & m_1 + m_2 \ar[ur]_{p_1 \tns p_2} & \\
}
\end{eqnarray}
Now, the equation associated with \eqref{eq:tensoredpb} is:
\begin{eqnarray*}
\lower23pt\hbox{\includegraphics[width=4cm]{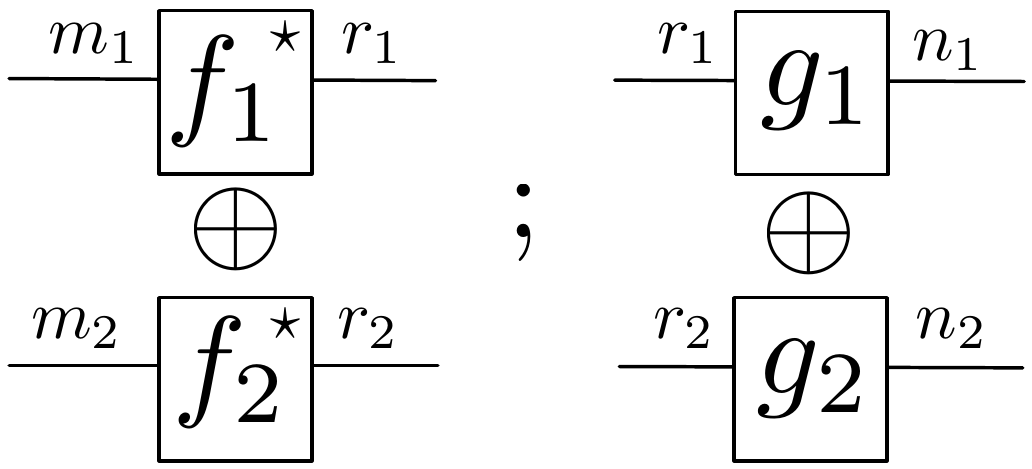}} & \qquad = \qquad
\lower23pt\hbox{\includegraphics[width=4cm]{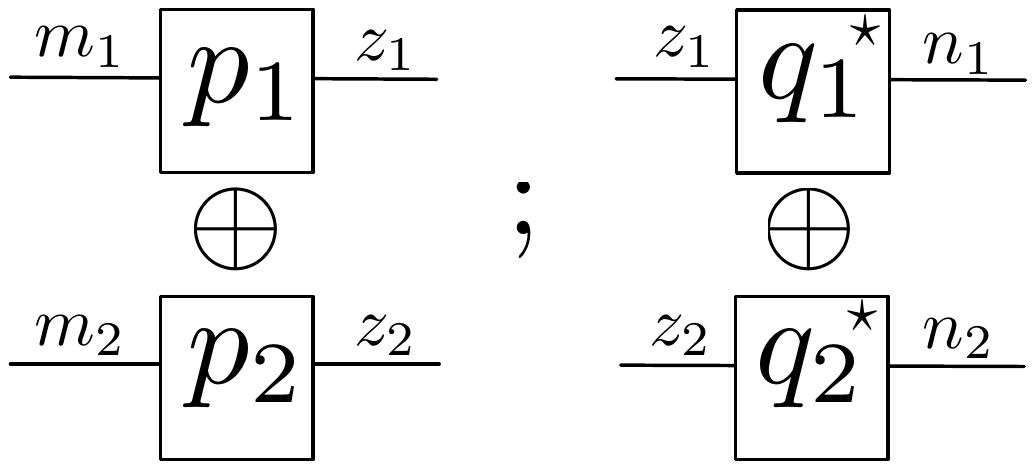}}
\end{eqnarray*}
which is clearly provable from the two equations given by assumption.
\end{proof}

\begin{construction} \label{constr:doublecube} Start with a pullback square (for which we fix notation $\midh$) where the cospan has carrier $k+1$, and consider the coproduct injections.
\begin{eqnarray*}
\xymatrix@=15pt{
& & & k \ar[dd]^{l} \\
\\
& n \ar[rr]^<<<<<<<<<<<<<{q} & & k+1 \\
r \ar[ur]^{g} \ar[rr]^<<<<<<<<<<<<<{f} & & m \ar[ur]_{p} & \\
& & & 1 \ar[uu]_{r}
}
\end{eqnarray*}
Build by pullback the front-rightmost (call $\frt$ the topmost, $\frbv$ the bottommost) and the rear-leftmost vertical faces (call $\rlt$ the topmost, $\rlb$ the bottommost).
\begin{eqnarray*}
\xymatrix@=15pt{
& r_k \ar[rr]^<<<<<<<<<<<<<{f_k} \ar[dd]^<<<<<<<<<{g_k} & & k \ar[dd]^{l} \\
& & r_k' \ar[dd]_<<<{f'_k} \ar[ur]_{g'_k} & \\
& n \ar[rr]^<<<<<<<<<<<<<{q} & & k+1 \\
r \ar[ur]^{g} \ar[rr]^<<<<<<<<<<<<<{f} & & m \ar[ur]_{p} & \\
& r_1' \ar[rr]^>>>>>>>{g'_1} \ar[uu]^<<<<<{f'_1}& & 1 \ar[uu]_{r} \\
& & r_1 \ar[uu]^>>>>>>>>>>>>{f_1} \ar[ru]_{g_1} &
}
\end{eqnarray*}
Then build by pullback the two missing front vertical faces (call $\flt$ the topmost, $\flb$ the bottommost).
\begin{eqnarray*}
\xymatrix@=15pt{
& r_k \ar[rr]^<<<<<<<<<<<<<{f_k} \ar[dd]^>>>>>>{g_k} & & k \ar[dd]^{l} \\
r_k'' \ar[dd]_{f''_k} \ar[rr]^>>>>>{g''_k} & & r_k' \ar[dd]_<<<{f'_k} \ar[ur]_{g'_k} & \\
& n \ar[rr]^<<<<<<<<<<<<<{q} & & k+1 \\
r \ar[ur]^{g} \ar[rr]^<<<<<<<<<<<<<{f} & & m \ar[ur]_{p} & \\
& r_1' \ar[rr]^>>>>>>>{g'_1} \ar[uu]^<<<<<{f'_1}& & 1 \ar[uu]_{r} \\
r_1'' \ar[uu]^{f''_1} \ar[rr]_{g''_1} & & r_1 \ar[uu]^>>>>>>>>>>>>{f_1} \ar[ru]_{g_1} &
}
\end{eqnarray*}
The arrows $h_k$ and $h_1$ completing the double cube are given by universal property of $r_k$ and $r_1$ respectively.
\begin{eqnarray}\label{eq:doublecubecoproductinj}
\xymatrix@=15pt{
& r_k \ar[rr]^<<<<<<<<<<<<<{f_k} \ar[dd]^>>>>>>{g_k} & & k \ar[dd]^{l} \\
r_k'' \ar[ur]^{h_k} \ar[dd]_{f''_k} \ar[rr]^>>>>>{g''_k} & & r_k' \ar[dd]_<<<{f'_k} \ar[ur]_{g'_k} & \\
& n \ar[rr]^<<<<<<<<<<<<<{q} & & k+1 \\
r \ar[ur]^{g} \ar[rr]^<<<<<<<<<<<<<{f} & & m \ar[ur]_{p} & \\
& r_1' \ar[rr]^>>>>>>>{g'_1} \ar[uu]^<<<<<{f'_1}& & 1 \ar[uu]_{r} \\
r_1'' \ar[uu]^{f''_1} \ar[rr]_{g''_1} \ar[ur]^>>>{h_1} & & r_1 \ar[uu]^>>>>>>>>>>>>{f_1} \ar[ru]_{g_1} &
}
\end{eqnarray}
Call $\rlb$ and $\rlt$ the bottommost rear left vertical face and the topmost rear left vertical face respectively. Also, let $\toph$ denote the topmost horizontal face and $\both$ the bottommost horizontal face.
\end{construction}

\begin{lemma} \label{lemma:pbdecomp} In diagram \eqref{eq:doublecubecoproductinj} all the faces are pullbacks and all the columns are coproduct injections.
\end{lemma}
\begin{proof} The only faces that are not pullbacks by construction are $\rlb$, $\rlt$, $\toph$ and $\both$. Let us prove that $\rlb$ is a pullback. Since $\flb$ and $\frbv$ are pullbacks, then the diagram given by pasting them together is also a pullback. By commutativity of the bottommost cube in \ref{eq:doublecubecoproductinj}, this is the same diagram as the one given by pasting together $\rlb$ and $\rrb$ which then is also a pullback. This, combined with the information that $\rrb$ is a pullback, gives that $\rlb$ is also a pullback.

Using pasting property of pullbacks in an analogous way, we can show that also $\rlt$, $\toph$ and $\both$ are pullbacks.

For the second part of the statement of the lemma, we can use the fact that $\F$ is an \emph{extensive} category \cite{CarboniLackWalters93ExtDistCats}. Now, since $l \: k \to k+1$ and $r \: 1 \to k+1$ are coproduct injections and $\frt$, $\frbv$ are pullbacks, then by extensivity also $f_1$ and $f'_k$ are coproduct injections. Similarly, the fact that $l,r$ are coproduct injections and $\rrt$, $\rrb$ are pullbacks implies that $g_k$ and $f'_1$ are coproduct injections. Finally, $f''_k$ and $f''_1$ are coproduct injections because $g_k$ and $f'_1$ are coproduct injections and $\rlt$, $\rlb$ are pullbacks.
\end{proof}

\begin{lemma} \label{lemma:coproductstablepullback} If the two leftmost diagrams below are pullbacks then the rightmost diagram is also a pullback.
\begin{eqnarray*}
\xymatrix@=15pt{
& \ar[dl]_{f_1} r_1 \ar[dr]^{g_1} & \\
n_1 \ar[dr]_{p_1} && m \ar[dl]^{q} \\
& z &
} \qquad \qquad
\xymatrix@=15pt{
& \ar[dl]_{f_2} r_2 \ar[dr]^{g_2} & \\
n_2 \ar[dr]_{p_2} && m \ar[dl]^{q} \\
& z &
} \qquad \qquad
\xymatrix@=15pt{
& \ar[dl]_{f_1 \tns f_2} r_1 + r_2 \ar[dr]^{[g_1, g_2]} & \\
n_1+n_2 \ar[dr]_{[p_1,p_2]} && m \ar[dl]^{q} \\
& z &
}
\end{eqnarray*}
\end{lemma}
\begin{proof} In $\F$ coproducts are stable under pullback.  \end{proof}

For the sequel we fix notation $\mu_n$ for the unique arrow from $n$ to $1$ in $\F$. If $n=2$, we just use the notation $\mu \: 2 \to 1$.

\begin{lemma}\label{lemma:pboneprovable} Let the following be a pullback square in $\F$. Then the corresponding circuit equation is provable in $\B$.
\begin{eqnarray*}
\xymatrix@=15pt{
& \ar[dl]_{f} r \ar[dr]^{g} & \\
n\ar[dr]_{p} && m \ar[dl]^{q} \\
& 1 &
}
\end{eqnarray*}
\end{lemma}
\begin{proof} In our argument we are going to consider pullbacks constructed in the canonical way suggested by Lemma \ref{lemma:coproductstablepullback}. This restriction is without loss of generality by virtue of Lemma \ref{lemma:mirrorcube}.

We reason by double induction on $n$ and $m$. If at least one between $n,m$ is $1$ or $0$, it easy to check that the statement holds. Thus we focus on the case $n,m \geq 2$.

\begin{itemize}
\item If $n =2$ and $m=2$, then the pullback square to consider is the one yielding the bialgebra equation that is an axiom of $\B$.

\item Fix $n+1$ and $m = 2$. In this case we need to consider the pullback for a cospan $n+1 \tr{\mu_{n+1}} 1 \tl{\mu} 2$. Using Lemma~\ref{lemma:coproductstablepullback}, we can first calculate the two leftmost pullbacks below. Then the rightmost is also a pullback for the desired cospan (observe that $\mu_{n+1} = \mu \circ (\mu_m \tns \id) = [\mu_m,\id]$ by uniqueness).
\begin{eqnarray*}
\xymatrix@=15pt{
& \ar[dl]_{f} r \ar[dr]^{g} & \\
n \ar[dr]_{\mu_n} && 2 \ar[dl]^{\mu} \\
& 1 &
} \qquad \qquad
\xymatrix@=15pt{
& \ar[dl]_{\mu}2\ar[dr]^{\id_2} & \\
1 \ar[dr]_{\id} && 2 \ar[dl]^{\mu} \\
& 1 &
} \qquad \qquad
\xymatrix@=15pt{
& \ar[dl]_{f \tns \mu}  r + 2 \ar[dr]^{[g, \id_2]} & \\
n+1 \ar[dr]_{[\mu_n,\id]} && 2 \ar[dl]^{\mu} \\
& 1 &
}
\end{eqnarray*}
We now show the proof of the equation associated with the rightmost diagram above.

\begin{center}[See derivation on scanned notes.]\end{center}
\item For the remaining inductive case, fix $n+1$ and $m+1$. The cospan of which we need to consider the pullback is $n+1 \tr{\mu_{n+1}} 1 \tl{\mu_{m+1}} m+1$. Again, Lemma~\ref{lemma:coproductstablepullback} tells us that the pullback is given the rightmost diagram below, on the base of the two leftmost pullback diagrams.
\begin{eqnarray*}
\xymatrix@=15pt{
& \ar[dl]_{f} r \ar[dr]^{g} & \\
n+1 \ar[dr]_{\mu_{n+1}} && m \ar[dl]^{\mu_m} \\
& 1 &
} \qquad \qquad
\xymatrix@=15pt{
& \ar[dl]_{\id_{n+1}}n+1\ar[dr]^{\mu_{n+1}} & \\
n+1 \ar[dr]_{\mu_{n+1}} && 1 \ar[dl]^{\id} \\
& 1 &
} \qquad \qquad
\xymatrix@=15pt{
& \ar[dl]_{[f,\id_{n+1}]}  r + (n+1) \ar[dr]^{g \tns \mu_{n+1}} & \\
n+1 \ar[dr]_{\mu_{n+1}} && m+1 \ar[dl]^{[\mu_m,\id]} \\
& 1 &
}
\end{eqnarray*}
We now show the proof of the equation associated with the rightmost diagram above.
\begin{center}[See derivation on scanned notes.]\end{center}
\end{itemize}

\end{proof}

We are now ready to show our completeness statement.

\begin{theorem} For all pullback squares of $\B$, the corresponding equation is provable in $\B$.
\end{theorem}
\begin{proof} Suppose that we want to prove the equation $c \approx c'$ associated with the pullback of a cospan $n \tr{p} z \tl{q} m$. Observe that $z$ can be written as a coproduct $\coprod_{1 \leq i \leq n} 1$. Thus by iteratively applying Construction \ref{constr:doublecube} the pullback of $\tr{p} \tl{q}$ can be decomposed into $z$ pullbacks of cospans with carrier $1$, giving raise to equations $c_1 \approx c'_1$, $\dots$, $c_z \approx c'_z$. By Lemma \ref{lemma:pbdecomp}, the double-cube diagrams that we obtain by applying Construction \ref{constr:doublecube} satisfy the assumptions of Lemma \ref{lemma:pbcoproductprovable}, that is, horizontal faces are pullbacks and columns are coproduct injections. Since by Lemma \ref{lemma:pboneprovable} $c_1 \approx c'_1$, $\dots$, $c_z \approx c'_z$ are all provable in $\B$, using the conclusion of Lemma \ref{lemma:pbcoproductprovable} we can then infer that $c \approx c'$ is also provable in $\B$. 
\end{proof}
