# Supplementary material for: Interacting Hopf Algebras: the theory of linear systems
Source: arXiv:1805.03032 source file (2018-05-04)
Supplement: Supplementary file 2 [file proofsABR.tex]

\begin{proof}[Proof of Lemma~\ref{lemma:threelaws}]
We construct the distributive law $\chi \: \wmon \bicomp{\Perm} \PROPR \To \PROPR \bicomp{\Perm} \wmon$ of statement $(a)$. As explained in the main text, statement $(b)$ follows.

For this purpose, it is first convenient to give an alternative characterisation of PROPs $\Mon$ and $\PROPR$: we make us of the fact that they are based on an \emph{algebraic} signature, i.e. one with all generators of coarity $1$. Consider the following grammars of terms:
\begin{align*}
 a,b & ::=&  x_i \mid \epsilon \mid a+b && i \in \N \\
 e & ::=& x_i \mid k \cdot e && i \in \N , k \in \PID
\end{align*}
We say that the first grammar generates\emph{$\Mon$-terms} and the second \emph{$\PROPR$-terms}. One should think of $(x_i)_{i \in \N}$ as a numerable set of variables and to $+$ and $\epsilon$ as a binary and a nullary operator playing the role of generators $\Wmult$ and $\Wunit$ respectively. The second grammar features for each $k \in \PID$ a unary operator $k \cdot$ intuitively corresponding to the generator $\scalar$ of $\PROPR$. We also introduce sets of equations
\begin{eqnarray}
 a+b = b+a \qquad (a+b)+c = a+(b+c) \qquad a+\epsilon = a \label{eq:axiomsAlgMon}\\
 k \cdot (l \cdot e) = kl \cdot e \qquad 1 \cdot e = e \label{eq:axiomsAlgPROPR}
\end{eqnarray}
where~\eqref{eq:axiomsAlgMon} mimics the equations of $\Mon$ and \eqref{eq:axiomsAlgPROPR} those of $\PROPR$. We now want to form PROPs where arrows are terms modulo equations. Whereas terms are going to be arrows $n \to 1$, to form arrows $n \to m$ we introduce the concept of linear list of terms. A \emph{linear list} $l^n_k$ is a list $[c_1,\dots,c_k]$ of (either $\Mon$- or $\PROPR$-) terms subject to the condition that only variables $x_1,\dots,x_n$ appear in $c_1,\dots,c_k$ and each of them appears exactly once.

We now call $\Mon'$ the PROP whose arrows $n \to m$ are linear lists $l^n_m$ of $\Mon$-terms modulo the equations~\eqref{eq:axiomsAlgMon}. The monoidal product is by concatenation of lists and composition is by substitution. Linear lists $n \to m$ of $\Mon'$ naturally correspond to string diagrams of $\Mon$. An example is given below, also showing composition in $\Mon'$ at work:

Generalising this example, one can easily check that $\Mon \cong \Mon'$. Similarly, one can form the PROP $\PROPR'$ whose arrows $n \to m$ are linear lists $l^n_m$ of $\PROPR$-terms modulo the equations~\eqref{eq:axiomsAlgPROPR}. Monoidal product and composition are defined as in $\Mon'$ and we have that $\PROPR' \cong \PROPR$.

In order to define a distributive law $\chi \: \wmon \bicomp{\Perm} \PROPR \To \PROPR \bicomp{\Perm} \wmon$, it thus suffices to define one $\chi' \: \wmon' \bicomp{\Perm} \PROPR' \To \PROPR' \bicomp{\Perm} \wmon'$. For this purpose, we observe that composable pairs $\tr{\in \wmon'}\tr{\PROPR'}$ are also captured by a grammar:
\begin{align*}
u & ::= & k \cdot u \mid a && k \in \PID
\end{align*}
The intuition is that a term $u$ cannot have a sub-term $k \cdot u_1$ nested inside a sub-term $u_2 + u_3$. Linear lists of terms generated by this grammar, which we call \emph{$\PROPR\Mon$-terms}, and quotiented by \eqref{eq:axiomsAlgMon}-\eqref{eq:axiomsAlgPROPR}, are in 1-1 correspondence with equivalence classes $[\tr{\in \wmon'}\tr{\PROPR'}]_{\equiv}$. An example is given below:

In a similar way we can capture the composable pairs $\tr{\in \PROPR'}\tr{\wmon'}$ in the target $\PROPR \bicomp{\Perm} \wmon$ of $\chi$:
\begin{align*}
&& w & ::= & \epsilon \mid w + w \mid e &&
\end{align*}
Terms generated by the above grammar are called \emph{$\Mon\PROPR$-terms}. Modulo the equations\eqref{eq:axiomsAlgMon}-\eqref{eq:axiomsAlgPROPR}, linear lists of $\Mon\PROPR$-terms are in 1-1 correspondence with equivalence classes $[\tr{\in \wmon'}\tr{\PROPR'}]_{\equiv}$. We are now ready to define our distributive law in an inductive way as a mapping of $\PROPR\Mon$-terms to $\Mon\PROPR$-terms:

One can verify that this 
\end{proof}
