# Supplementary material for: Interacting Hopf Algebras: the theory of linear systems
Source: arXiv:1805.03032 source file (2018-05-04)
Supplement: Supplementary file 3 [file appendixCospanF.tex]

We claim that $\FROB$ is a presentation of $\Cospan{\F}$.
 \begin{theorem}\label{th:FROBcomplete} $\FROB \cong \Cospan{\F}$. \end{theorem}
 For this purpose, we need to check that the equation associated with any pushout diagram in $\F$ is provable by the axioms of $\FROB$. The key observation is that we can confine ourselves to just pushouts involving the basic operations of $\wmon$. More formally, we call \emph{atomic} any circuit of $\wmon$ of shape $f \poi b \poi g$, where $f$ and $g$ consist of circuits $\Idnet$ and $\symNet$ composed together via $\tns$ or $\poi$, and $b$ is either $\id_0$ or an operation in the signature of $\wmon$. Completeness for atomic circuits will be pivotal in the proof of Theorem~\ref{th:FROBcomplete}.
 \begin{lemma}\label{lemma:atomicCircuits} Let $\tl{f} \tr{g}$ be a span in $\F$ where $f$ and $g$ are in the image of atomic circuits and suppose that the following is a pushout square.
  \[ \xymatrix@=10pt{ & \ar[dl]_{f} r \ar[dr]^{g} & \\
 \ar[dr]_{p} m & & \ar[dl]^{q} n \\
 & z & } \]
 Then:
\begin{enumerate}
  \item $p$ and $q$ are also in the image of atomic circuits;
   \item the associated equation is provable in $\FROB$.
  \end{enumerate}
 \end{lemma}
 \begin{proof}
 The two points are proved by case analysis on all the possible interactions of operations of $\wmon$ and $\bcom$.
 \end{proof}
 We can now provide a proof of Theorem~\ref{th:FROBcomplete}.

 \begin{proof}[Proof of Theorem~\ref{th:FROBcomplete}] Let the following be a pushout square in $\F$.
 \begin{equation}\label{eq:poFROBcompl}
  \vcenter{\xymatrix@=10pt{ & \ar[dl]_{f} r \ar[dr]^{g} & \\
 \ar[dr]_{p} m & & \ar[dl]^{q} n \\
 & z & }}
 \end{equation}
Pick expansions $f = f_1 \poi \dots \poi f_k$ and $g = g_1 \poi \dots \poi g_j$, with each $f_i$ and $g_i$ in the image of an atomic circuit. We can calculate the pushout above by tiling pushouts of atomic circuits as follows:
  \begin{equation}\label{eq:poatomicexpansion}
  \vcenter{ \xymatrix@R=2pt{
&&&\ar[dl]_{f_1} z \ar[dr]^{g_1} &&& \\
&& \ar[dl]_{f_2} \ar[dr] && \ar[dl] \ar[dr]^{g_2} &&\\
& \dots\ar[dl]_{f_k} \ar[dr] &&\ar[dr] \ar[dl] &&\dots \ar[dl] \ar[dr]^{g_j} &\\
\ar[dr] &&&\dots &&& \ar[dl] \\
&\ar[dr] &&\ar[dl]\dots \ar[dr]&& \ar[dl] &\\
&&\dots\ar[dr] && \dots\ar[dl] &&\\
&&&&&&
}
}
 \end{equation}
 Point 1 of Lemma~\ref{lemma:atomicCircuits} guarantees that each inner square only involves arrows in the image of some atomic circuit and Point 2 ensures that all the associated equations are provable in $\FROB$. It follows that also the equation associated with the outer pushout~\eqref{eq:poatomicexpansion} is provable. By Lemma~\ref{lemma:mirrorcube}, the equation for~\eqref{eq:poFROBcompl} is equivalent to the one for~\eqref{eq:poatomicexpansion} because they are pushouts for the same span. Therefore the latter is also provable in $\FROB$. \end{proof}
